# Supplementary material for: Multi-scale Matching Networks for Semantic Correspondence
Source: arXiv:2108.00211 source file (2021-08-27)
Supplement: Supplementary file 1 [file supp.pdf]

# Supplement Material

## 1. Parameter Table

Images are resized to  $224 \times 320$  for all datasets both in training and testing.

|                  |                                                                                                         | ResNet-50                                             | ResNet-101           | ResNeXt-101        | ResNet-101-FCN      |
|------------------|---------------------------------------------------------------------------------------------------------|-------------------------------------------------------|----------------------|--------------------|---------------------|
| Conv Intra-fused | conv: output channel = 21, kernel size = $1 \times 1$ , stride = 1                                      |                                                       |                      |                    |                     |
| Conv Cross-fused | conv: output channel = 21, kernel size = $3 \times 3$ , stride = 1, padding = 1                         |                                                       |                      |                    |                     |
| Deconv           | transpose conv: output channel = 21, kernel size = $4 \times 4$ , stride = 2, padding = 1, bias = False |                                                       |                      |                    |                     |
| LSA              | conv_key                                                                                                | conv: output channel = 10, kernel size = $1 \times 1$ |                      |                    |                     |
|                  | conv_value                                                                                              | conv: output channel = 10, kernel size = $1 \times 1$ |                      |                    |                     |
|                  | conv_query                                                                                              | conv: output channel = 10, kernel size = $1 \times 1$ |                      |                    |                     |
|                  | conv_aggregate                                                                                          | conv: output channel = 21, kernel size = $1 \times 1$ |                      |                    |                     |
| # Params         | backbone                                                                                                | $25.6 \times 10^6$                                    | $44.5.0 \times 10^6$ | $88.8 \times 10^6$ | $54.4 \times 10^6$  |
|                  | MMNet w/o backbone                                                                                      | $4.8 \times 10^6$                                     | $10.3 \times 10^6$   | $10.3 \times 10^6$ | $10.3 \times 10^6$  |
|                  | MMNet                                                                                                   | $30.4 \times 10^6$                                    | $54.8 \times 10^6$   | $99.1 \times 10^6$ | $64.7 \times 10^6$  |
| FLOPs            | backbone                                                                                                | $11.8 \times 10^9$                                    | $22.4 \times 10^9$   | $47.0 \times 10^9$ | $127.6 \times 10^9$ |
|                  | MMNet w/o backbone                                                                                      | $3.1 \times 10^9$                                     | $4.6 \times 10^9$    | $4.6 \times 10^9$  | $12.7 \times 10^9$  |
|                  | MMNet                                                                                                   | $14.9 \times 10^9$                                    | $27.0 \times 10^9$   | $51.6 \times 10^9$ | $140.3 \times 10^9$ |

Table 1: Implementation details of MMNet, and numbers of parameters and FLOPs introduced by different modules. In this table, ‘*Conv Intra-fused*’ and ‘*Conv Cross-fused*’ denote the convolution operation in the intra-scale and cross-scale feature enhancements separately, ‘*Deconv*’ indicates the deconvolution operation to upscale the feature maps during the cross-scale feature enhancement, and ‘*LSA*’ is short for the local self attention module used at the end of the intra-scale feature enhancement.

**Analysis.** MMNet introduces additional parameters only in its feature enhancement module. We follow BDCN to set the parameters of scale enhancement modules. Each scale enhancement module contains four  $3 \times 3$  convolution operations with dilation 1, 4, 8, 12 respectively. The output channel numbers of these convolution operations are set to 32. The output channel numbers of other convolution and deconvolution operations are set to 21 to reduce the computational cost. We compare the additional parameters and FLOPs introduced by MMNet with four different backbones including ResNet-50, ResNet-101, ResNeXt-101 and ResNet-101-FCN. The additional parameters are no larger than 25% of that of any backbone. For the FLOPs, we add at most 26.3% computational cost when using ResNet-50 as the backbone.

## 2. Additional Results

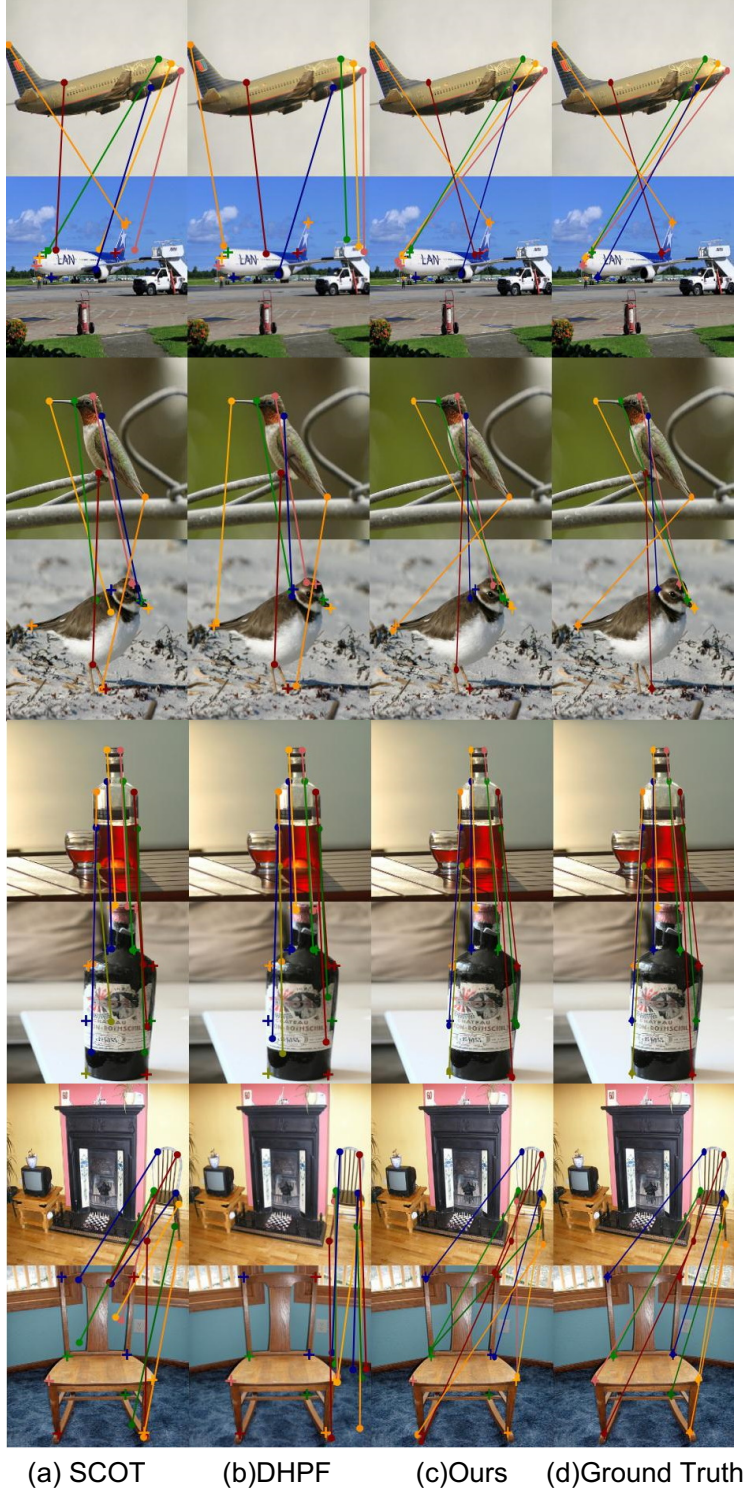

Figure 1: Key-point matching results on SPair-71k dataset compared with SCOT and DHPF. The odd rows are the source images, and the even rows are the target images. Destination key points are denoted with crosses.

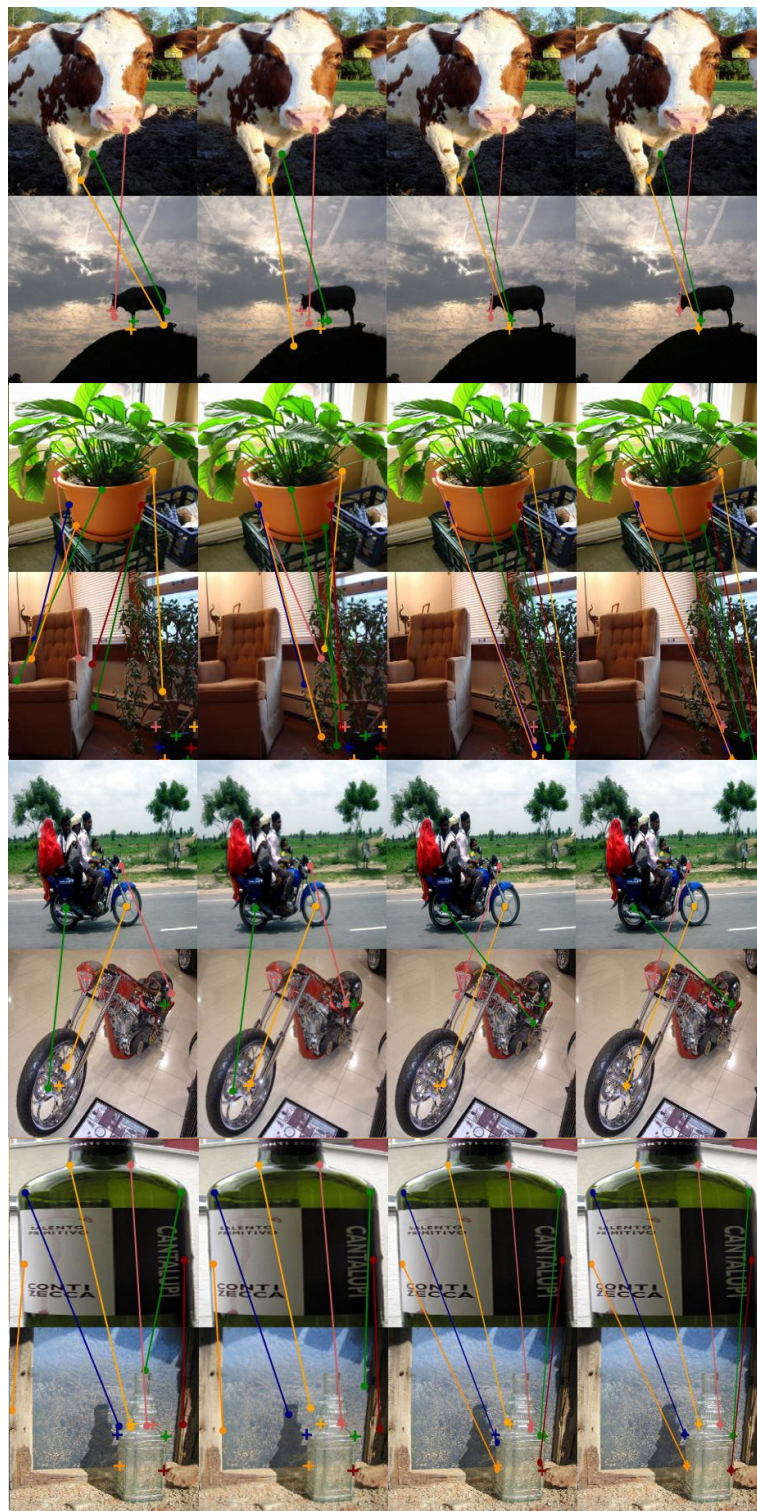

(a) SCOT      (b) DHPF      (c) Ours      (d) Ground Truth

Figure 2: Key-point matching results on SPair-71k dataset compared with SCOT and DHPF . The odd rows are the source images, and the even rows are the target images. Destination key points are denoted with crosses.



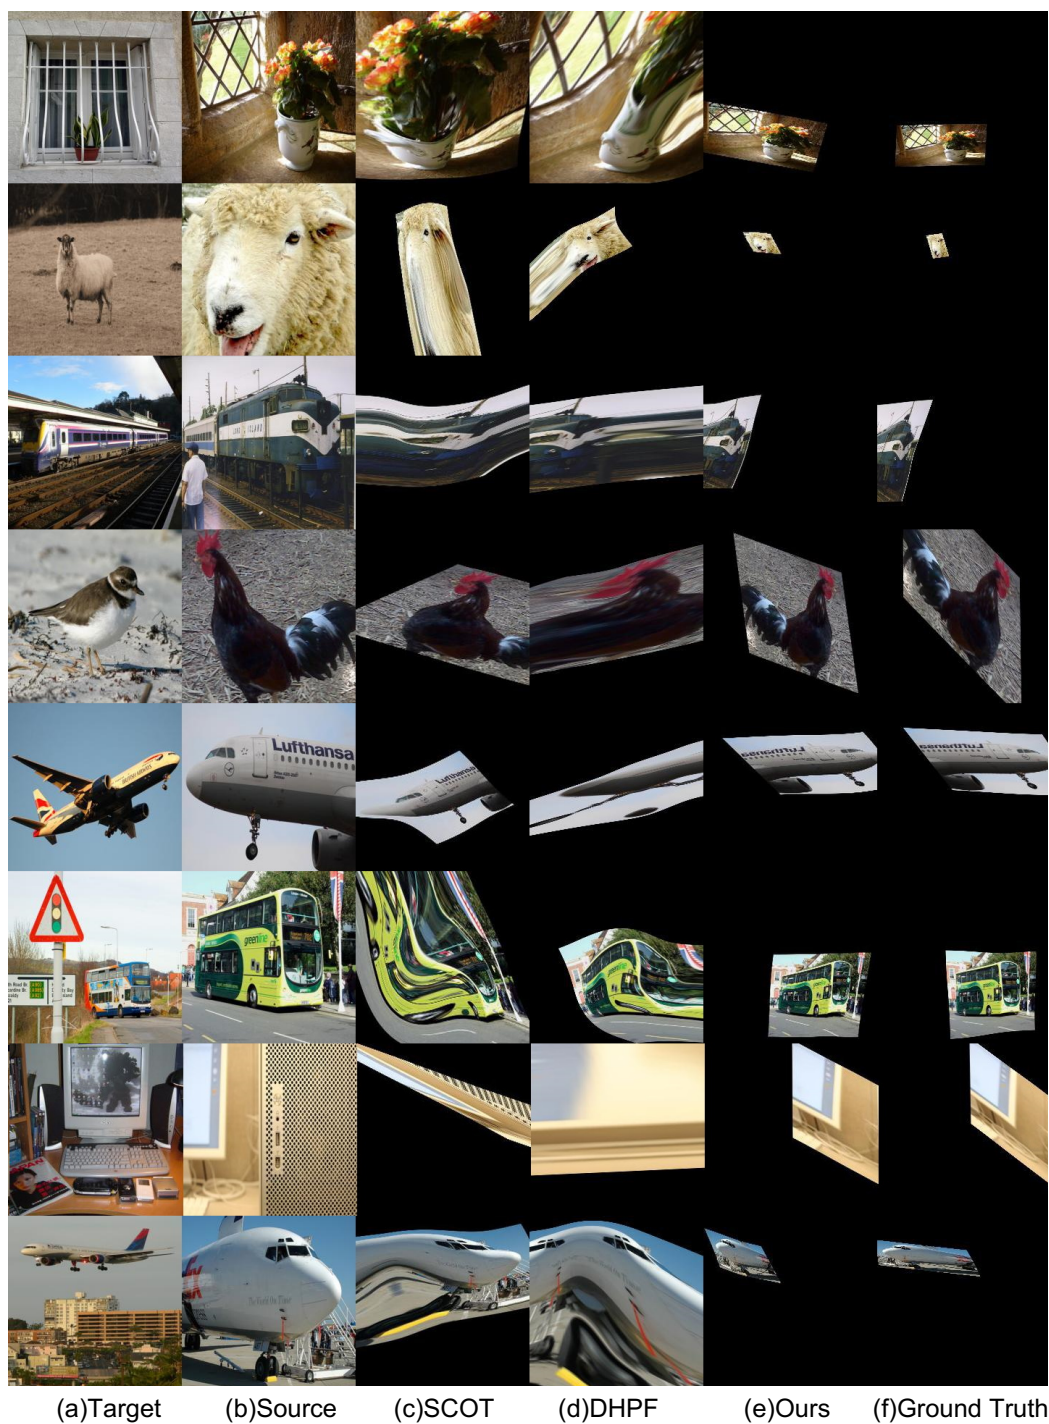

Figure 3: Warped images by thin-plate splines with the predicted key point pairs on SPair-71k dataset compared with SCOT and DHPF



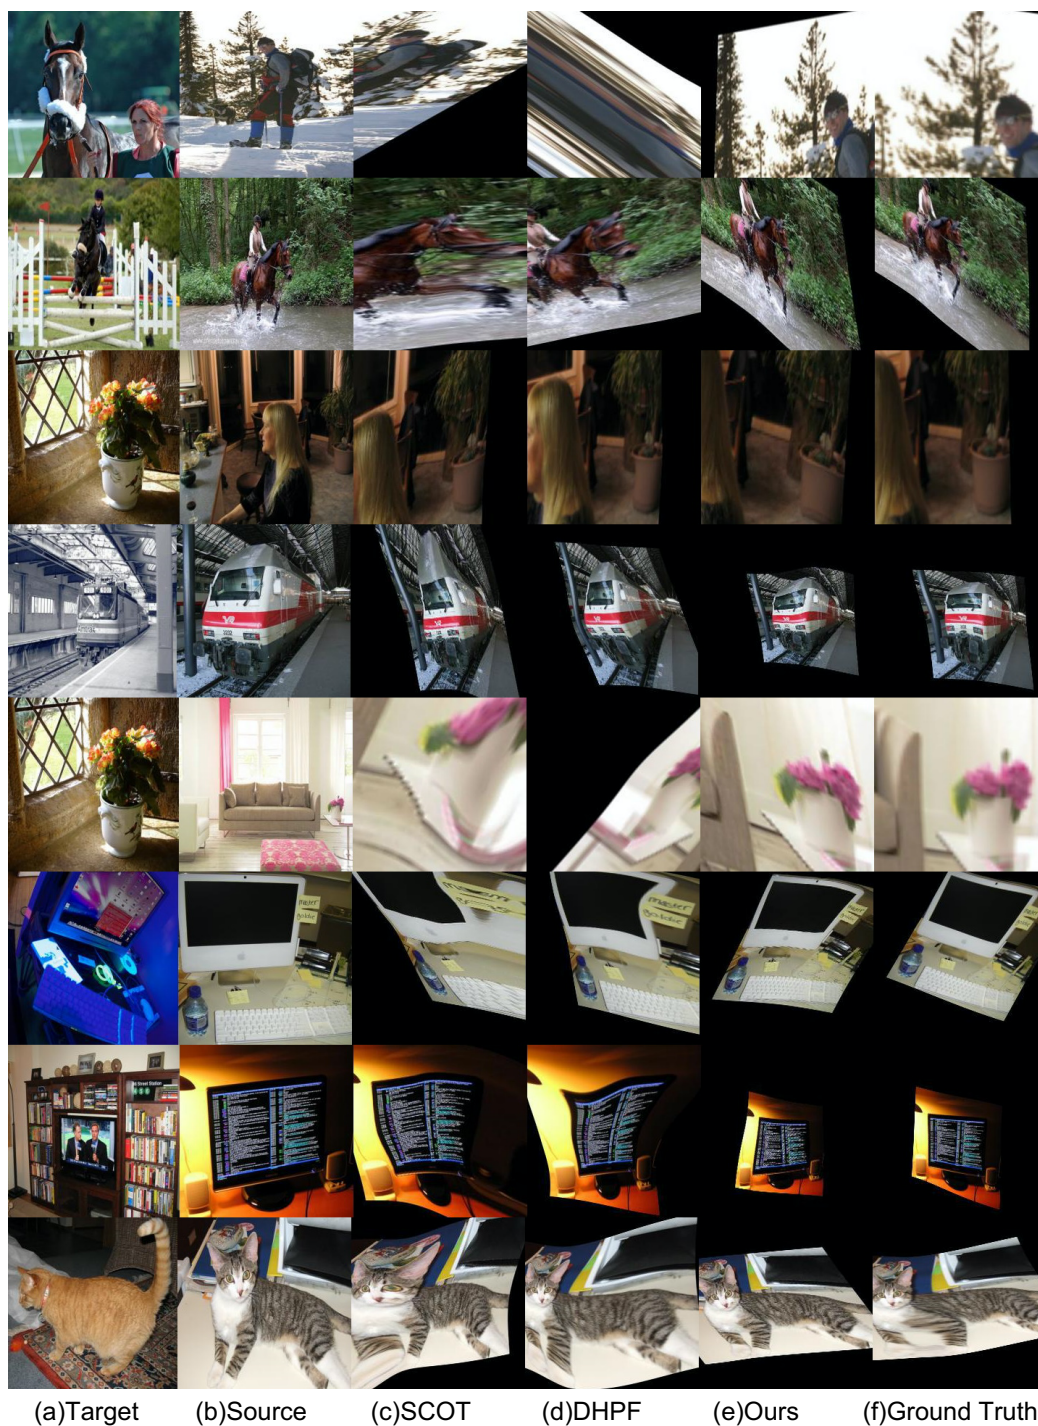

Figure 4: Warped images by thin-plate splines with the predicted key point pairs on SPair-71k dataset compared with SCOT and DHPF
